# Supplementary material for: Generative deep learning for decision making in gas networks
Source: arXiv:2102.02125 source file (2021-02-03)
Supplement: Supplementary file 1 [file Formulation.tex]

\begin{align*}
  \min \sum_{t\in\setTimestepsNoZero} \bigg(
   & \big(\granularity{t}-\granularity{t-1}\big)
   \sum_{v\in\setBoundaryNodes} \big(\paramCostSlackP \cdot (\varSlackPressurePos{v}{t} + \varSlackPressureNeg{v}{t}) + \paramCostSlackQ \cdot (\varSlackFlowPos{v}{t} + \varSlackFlowNeg{v}{t})\big) \\
  &+ \paramCostOpModes\cdot\varOpModeChange{t} \\
  &+ \sum_{a\in\setRegulators} \paramCostRgModeChanges\cdot\varRegModeChange{a}{t} \\
  &+ \sum_{u\in\setCompressorUnits{a}, a\in\setCompressorStations} \paramCostUnitStarts\cdot\varUnitStart{u}{t} \\
  &+ \sum_{a\in\setRegulators} \big( \paramCostRgPLChanges\cdot\varRgPLChange{a}{t} + \paramCostRgPRChanges\cdot\varRgPRChange{a}{t} + \paramCostRgQChanges\cdot\varRgQChange{a}{t} \big) \\
  &+ \sum_{a\in\setCompressorStations} \big( \paramCostCsPLChanges\cdot\varCsPLChange{a}{t} + \paramCostCsPRChanges\cdot\varCsPRChange{a}{t} + \paramCostCsQChanges\cdot\varCsQChange{a}{t} \big)\bigg) \\
  % pipes
  \text{s.t.} \qquad \qquad \forall t\in\setTimestepsNoZero \quad \forall a\in\setPipes \qquad
  0 &= \varPressure{l}{t} + \varPressure{r}{t} - \varPressure{l}{t-1} - \varPressure{r}{t-1}
    + \frac{2\specificGasConstant\generalGasTemperature\compressibilityFactor{a}(\granularity{t} - \granularity{t-1})}{\pipeLength{a}\pipeArea{a}}
      \left(\varPipeFlow{r}{a}{t} - \varPipeFlow{l}{a}{t}\right) \\
  0 &= \varPressure{r}{t} - \varPressure{l}{t} + \frac{\frictionFactor{a}\pipeLength{a}}{4\pipeDiameter{a}\pipeArea{a}}
       \left(\paramAbsoluteVelocity{l}{a}\varPipeFlow{l}{a}{t} + \paramAbsoluteVelocity{r}{a}\varPipeFlow{r}{a}{t}\right)
       + \frac{\gravitationalAcceleration\pipeSlope{a}\pipeLength{a}}{2\specificGasConstant\generalGasTemperature\compressibilityFactor{a}}
               \left(\varPressure{l}{t} + \varPressure{r}{t}\right) \\
  % resistors
  \forall t\in\setTimestepsNoZero \quad \forall a\in\setResistors \qquad
  \varPressure{l}{t} - \varPressure{r}{t} &= \frac{\resistorDragFactor{a}\paramAbsoluteVelocityI{a}}{2\pipeArea{a}}\varArcFlow{a}{t} \\
  % valves
  \forall t\in\setTimestepsNoZero \quad \forall a\in\setValves \qquad
  \varPressure{l}{t} - \varPressure{r}{t} &\leq ( 1 - \varModeOpen{a}{t} )(\paramPressureUB{l}{t}-\paramPressureLB{r}{t}) \\
  \varPressure{l}{t} - \varPressure{r}{t} &\geq ( 1 - \varModeOpen{a}{t} )(\paramPressureLB{l}{t}-\paramPressureUB{r}{t}) \\
  \varArcFlow{a}{t} &\leq ( \varModeOpen{a}{t} )\paramArcFlowUB{a}{t} \\
  \varArcFlow{a}{t} &\geq ( \varModeOpen{a}{t} )\paramArcFlowLB{a}{t} \\
  \varModeOpen{a}{t} &= \sum_{o\in\setNSModes : M(o,a)=\text{op}} \varNSmode{o}{t} \\
  % regulators
  \forall t\in\setTimestepsNoZero \quad \forall a\in\setRegulators \qquad \qquad \qquad
  1 &= \varModeClosed{a}{t} + \varModeBypass{a}{t} + \varModeActive{a}{t}\\
  \varPressure{l}{t} - \varPressure{r}{t} &\leq  + ( 1 - \varModeBypass{a}{t} )(\paramPressureUB{l}{t}-\paramPressureLB{r}{t}) \\
  \varPressure{l}{t} - \varPressure{r}{t} &\geq  + ( 1 - \varModeBypass{a}{t} - \varModeActive{a}{t} )(\paramPressureLB{l}{t}-\paramPressureUB{r}{t}) \\
  q_a &\leq ( 1 - \varModeClosed{a}{t} )\paramArcFlowUB{a}{t} \\
  q_a &\geq 0
\end{align*}
\begin{align*}
  % compressors
  \forall t\in\setTimestepsNoZero \quad \forall a\in\setCompressorStations & \\
  1 &= \sum_{c\in\setCompressorConfigurations{a}} \varModeConfiguration{c}{a}{t} + \varModeBypass{a}{t} + \varModeClosed{a}{t} \\
  \varPressure{l}{t} &= \varBypassPressure{a}{t} + \varClosedPressureL{a}{t} + \sum_{c\in\setCompressorConfigurations{a}} \varConfigPressureL{c}{a}{t} \\
  \varPressure{r}{t} &= \varBypassPressure{a}{t} + \varClosedPressureR{a}{t} + \sum_{c\in\setCompressorConfigurations{a}} \varConfigPressureR{c}{a}{t} \\
  \varArcFlow{a}{t} &= \varBypassFlow{a}{t} + \sum_{c\in\setCompressorConfigurations{a}} \varConfigFlow{c}{a}{t} \\
  \varConfigPressureLLB{c}{a}{t}\varModeConfiguration{c}{a}{t} \leq \makebox[\myLength][r]{\varConfigPressureL{c}{a}{t}} &\leq \varConfigPressureLUB{c}{a}{t}\varModeConfiguration{c}{a}{t} \quad \forall c\in\setCompressorConfigurations{a} \\
  \varConfigPressureRLB{c}{a}{t}\varModeConfiguration{c}{a}{t} \leq \makebox[\myLength][r]{\varConfigPressureR{c}{a}{t}} &\leq \varConfigPressureRUB{c}{a}{t}\varModeConfiguration{c}{a}{t} \quad \forall c\in\setCompressorConfigurations{a} \\
  \varConfigFlowLB{c}{a}{t}\varModeConfiguration{c}{a}{t} \leq \makebox[\myLength][r]{\varConfigFlow{c}{a}{t}} &\leq \varConfigFlowUB{c}{a}{t}\varModeConfiguration{c}{a}{t} \quad \forall c\in\setCompressorConfigurations{a} \\
  \varBypassPressureLB{a}{t}\varModeBypass{a}{t} \leq \makebox[\myLength][r]{\varBypassPressure{a}{t}} &\leq \varBypassPressureUB{a}{t}\varModeBypass{a}{t} \\
  \varBypassFlowLB{a}{t}\varModeBypass{a}{t} \leq \makebox[\myLength][r]{\varBypassFlow{a}{t}} &\leq \varBypassFlowUB{a}{t}\varModeBypass{a}{t} \\
  \varClosedPressureLLB{a}{t}\varModeClosed{a}{t} \leq \makebox[\myLength][r]{\varClosedPressureL{a}{t}} &\leq \varClosedPressureLUB{a}{t}\varModeClosed{a}{t} \\
  \varClosedPressureRLB{a}{t}\varModeClosed{a}{t} \leq \makebox[\myLength][r]{\varClosedPressureR{a}{t}} &\leq \varClosedPressureRUB{a}{t}\varModeClosed{a}{t} \\
  w\cdot \varConfigPressureL{c}{a}{t} + x\cdot \varConfigPressureR{c}{a}{t} + y\cdot \varConfigFlow{c}{a}{t} + z\varModeConfiguration{c}{a}{t} &\leq 0 \quad \forall (w,x,y,z) \in\setConfigurationFacets{c} \quad \forall c\in\setCompressorConfigurations{a} \\
  \varModeBypass{a}{t} &= \sum_{o\in\setNSModes : M(o,a)=\text{by}} \varNSmode{o}{t} \\
  \varModeClosed{a}{t} &= \sum_{o\in\setNSModes : M(o,a)=\text{cl}} \varNSmode{o}{t} \\
  \varModeConfiguration{c}{a}{t} &= \sum_{o\in\setNSModes : M(o,a)=c}   \varNSmode{o}{t} \quad\forall c\in\setCompressorConfigurations{a} \\
  \forall t\in\setTimestepsNoZero \qquad
  1 &= \sum_{o \in \setNSModes} \varNSmode{o}{t} \\
  1 &= \sum_{\flowDirection \in \setFlowDirectionsNavi} \varNSflowdir{f}{t}
\end{align*}
\begin{align*}
  % boundary nodes
  \forall t\in\setTimestepsNoZero \quad \forall v\in\setBoundaryNodes \qquad
  0 &= \sum_{(l,v)=a\in\setPipes} \varPipeFlow{v}{a}{t} - \sum_{(v,r)=a\in\setPipes} \varPipeFlow{v}{a}{t} \\
    &+ \sum_{(l,v)=a\in\setArcs\setminus\setPipes} \varArcFlow{a}{t} - \sum_{(v,r)=a\in\setArcs\setminus\setPipes} \varArcFlow{a}{t} + \varInflowValue{v}{t} \\
  \varInflowValue{v}{t} &\geq ( 1 - \sum_{\flowDirection=(\flowDirectionEntries, \flowDirectionExits)\in\setFlowDirectionsNavi : v\not\in\flowDirectionExits}  \varNSflowdir{\flowDirection}{t})\paramInflowValueLB{v}{t}\\
  \varInflowValue{v}{t} &\leq ( 1 - \sum_{\flowDirection=(\flowDirectionEntries, \flowDirectionExits)\in\setFlowDirectionsNavi : v\not\in\flowDirectionEntries} \varNSflowdir{\flowDirection}{t})\paramInflowValueUB{v}{t} \\
  \demandPressure{v}{t} &= \varPressure{v}{t} - \varSlackPressurePos{v}{t} + \varSlackPressureNeg{v}{t} \\
  % inner nodes
  \forall t\in\setTimestepsNoZero \quad \forall v\in\setInnerNodes \qquad
  0 &= \sum_{(l,v)=a\in\setPipes} \varPipeFlow{v}{a}{t} - \sum_{(v,r)=a\in\setPipes} \varPipeFlow{v}{a}{t}\\
    &+ \sum_{(l,v)=a\in\setArcs\setminus\setPipes} \varArcFlow{a}{t} - \sum_{(v,r)=a\in\setArcs\setminus\setPipes} \varArcFlow{a}{t} \\
  % operation modes
  \forall t\in\setTimestepsNoZero \quad \forall o\in\setNSModes \qquad
  \varNSmode{o}{t} &\leq \sum_{(o,\flowDirection)\in\setNSValidPairs} \varNSflowdir{\flowDirection}{t} \\
  % exit pressures
  \forall t\in\setTimestepsNoZero \quad \forall v\in\setBoundaryNodesExitP \qquad
  \varPressure{v}{t} &\leq \paramPressureUBExitFenceGroup{v} + ( 1 - \sum_{\flowDirection=(\flowDirectionEntries, \flowDirectionExits)\in\setFlowDirectionsNavi : v\in\flowDirectionExits} \varNSflowdir{\flowDirection}{t})(\paramPressureUB{v}{t} - \paramPressureUBExitFenceGroup{v}) \\
  % flow dir conditions
  \forall t\in\setTimestepsNoZero \quad \forall (f,\setVertices^{w_1},\setVertices^{w_2}) \in \setFlowDirectionConditions \qquad
  0 &\leq (1 - \varNSflowdir{f}{t})C_1
          - \sum_{v \in \setVertices^{w_1}} \text{sgn}(f,v) \varInflowValue{v}{t}
          + \sum_{v \in \setVertices^{w_2}} \text{sgn}(f,v) \varInflowValue{v}{t} \\
  % fence groups
  \forall t\in\setTimestepsNoZero \quad \forall g\in\setNSFenceGroups \qquad
  \demandInflow{g}{t} &= \sum_{v\in g}\left( \varInflowValue{v}{t} - \varSlackFlowPos{v}{t} + \varSlackFlowNeg{v}{t} \right)
\end{align*}
